# Supplementary material for: Joint spatial filter and time-varying MCLP for dereverberation and interference suppression of a dynamic/static speech source
Source: arXiv:1910.09782 source file (2019-10-22)
Supplement: Supplementary file 1 [file appendix.tex]

\subsection{Joint posterior $\Probability{ \bld{g}_{m,n},\bld{g}_{m,n-1} \given \bld{X}_{0:n} }$}
The joint posterior is also a Gaussian distribution
\begin{equation}
\mathcal{N}_c\inBrackets{ 
		\begin{bmatrix}
			\bs{\mu}_{m,n-1\given n}\\
			\bs{\mu}_{m,n\given n}
		\end{bmatrix},
		\begin{bmatrix}
			\bs{\Sigma}_{n-1\given n}\hspace{20pt}\bs{\Sigma}_{n\given n}^T \bld{J}_{n-1}^T\\
			\bld{J}_{n-1}\bs{\Sigma}_{n\given n}\hspace{20pt}\bs{\Sigma}_{n\given n}
		\end{bmatrix}
		 },
\end{equation}
where $\bld{J}_{n-1} = \bs{\Sigma}_{n-1\given n-1} \bs{\Sigma}_{n\given n-1}^{-1} $.
\begin{equation}
	\bs{\mu}_{m,n-1\given n} = \bs{\mu}_{m,n-1\given n-1} + \bld{J}_{n-1} \inBrackets{ \bs{\mu}_{m,n\given n} - \bs{\mu}_{m,n-1\given n-1} }
\end{equation}
\begin{equation}
	\bs{\Sigma}_{n-1|n} = \bs{\Sigma}_{n-1|n-1} - \bld{J}_{n-1} \inBrackets{ \bs{\Sigma}_{n|n}- \bs{\Sigma}_{n|n-1}}.
\end{equation}
Consider 
\begin{multline}
	\hspace{-10pt}
	\Expectation{ \inBrackets{ \bld{g}_{m,n} - \bld{g}_{m,n-1} } \inBrackets{ \bld{g}_{m,n} - \bld{g}_{m,n-1} }^H } = 
	\Expectation{ \bld{g}_{m,n} \bld{g}_{m,n}^H}\\-\Expectation{ \bld{g}_{m,n} \bld{g}_{m,n-1}^H} - \Expectation{ \bld{g}_{m,n-1} \bld{g}_{m,n}^H}+\Expectation{ \bld{g}_{m,n-1} \bld{g}_{m,n-1}^H}.
\end{multline}
\begin{equation}
	\Expectation{ \bld{g}_{m,n} \bld{g}_{m,n}^H} = \bs{\Sigma}_{n|n} + 
\end{equation}
